# Supplementary material for: High-Precision Extraction of Emerging Concepts from Scientific Literature
Source: arXiv:2006.06877 source file (2020-06-11)
Supplement: Supplementary file 1 [file appendix_anno.tex]

\section{Annotation instructions}
\label{appendix:anno}
A cluster of phrases that corresponds to a concept is a positive. A concept is something that multiple researchers would be interested in having a page for. Concepts can be methods, datasets, tasks, problem spaces, fields of research, phenomena or mathematical objects that people study, etc. It can be difficult to tell when a potential concept is too specific or too general. When a potential concept is a phrase with many general uses, it is likely not a concept (e.g. \emph{sentence}). If a word is a technical word, but a page for it would require more specificity, it is likely not a concept. \emph{Sentence} is not a concept, but \emph{sentence representations} or \emph{criminal sentencing} or \emph{linguistic sentence structure} all could be. When a potential concept has extra adjectives, it can be a difficult decision, but it is often not a concept (e.g. \emph{robust PCA} is a concept, but \emph{efficient neural networks} is not. \emph{Robust PCA} is the name of a method, whereas \emph{efficient} is a generic adjective in this case). If a paper introduces a new method, dataset, task, etc, that new thing is likely a concept, but just introducing a new phrase does not qualify the phrase as a concept. Additionally, just because something can be defined does not make it a concept. It needs to also have people doing research with it or about it.

When annotating, go through a few steps before deciding that something is not a concept. Going through each step is important, because things that may seem obvious are often not. For example, to a layperson, it may be obvious that \emph{BERT} is not a concept (it looks like a person's name or a Sesame Street character), but after inspecting a couple of papers, it is clear that \emph{BERT} is a new method. These steps are: (1) Look at the phrase (2) Look at the linked "central" paper, and perhaps its citations (3) Look at other papers that mention the phrase (4) Search Google for the phrase (5) Annotate.

Sometimes the noun phrase cluster represents an incomplete noun phrase. Maybe someone introduced a new method called \emph{Wildly Efficient Neural Networks}, but a noun phrase extraction failure resulted in the extraction of \emph{Wildly Efficient Neural}. We consider this case a good concept, only if the actual extraction is extremely unlikely to occur in a different context. As a negative example, if \emph{neural networks} is a good concept, but a noun phrase cluster just contains the word \emph{neural}, this would not be considered a good concept, because \emph{neural} appears in many other contexts, and is not a good concept on its own.
